# Supplementary material for: Purely magnetic logic based on polarized spin waves
Source: arXiv:1906.08702 ancillary file (2019-06-20)
Supplement: Supplementary file 1 [file SM.pdf]

# Supplementary Materials for

## Purely magnetic logic based on polarized spin waves

**Authors:** Weichao Yu,[1] Jin Lan,[1] Jiang Xiao[1,2*]

**Affiliations:**

[1] State Key Laboratory of Surface Physics and Department of Physics, Fudan University, Shanghai 200433, China.

[2] Institute for Nanoelectronics Devices and Quantum Computing, Fudan University, Shanghai 200433, China.

*Correspondence to: xiaojiang@fudan.edu.cn

**This PDF file includes:**

1. Numerical Method
2. Logic gates based on double-threshold non-linearity
3. Fulfillment of five essential characteristics for scalable computing
4. Operation steps of 4-bit adder
5. Descriptions for Movies S1 to S3

**Other Supplementary Materials for this manuscript includes the following:**

Movies S1 to S3

## 1. Numerical Method

Modelling

The functionalities of the proof-of-principle logic gates are verified via micromagnetic simulations. The simulations are performed in a two-dimensional environment built upon a self-developed Micromagnetic Module in COMSOL Multiphysics (a commercial software based on finite element method), where the Landau-Lifshitz-Gilbert (LLG) equation is transformed into weak form, and solved with a generalized alpha method (*1*-*3*). Strict benchmarking has been performed to ensure the correctness and robustness of this Micromagnetic Module. In comparison with the existing micromagnetic packages (such as MuMax or OOMMF), the advantage of this COMSOL-based Micromagnetic Module lies in that the it can easily deal with complicated device structures such as the ones studied in this paper. The same method has been applied in several cases, including both ferromagnetic and antiferromagnetic systems (*4*-*7*).

The magnetization dynamics of the SyAF structure is described by the coupled Landau-Lifshitz-Gilbert (LLG) equations for each sub-layer (*6, 8*),

$$\dot{\mathbf{m}}_j(\mathbf{r},t) = -\gamma \mathbf{m}_j(\mathbf{r},t) \times \mathbf{H}_j^{\mathrm{eff}} + \alpha_j \mathbf{m}_j(\mathbf{r},t) \times \dot{\mathbf{m}}_j(\mathbf{r},t) + \boldsymbol{\tau}_j,$$

where $j = 1, 2, 3$ denotes the lower and upper layer of the logic track and the memory track above, respectively. Here $\gamma = 2.21\times10^5$ Hz·m/A is the gyromagnetic ratio, $\alpha_j$ is the Gilbert damping constant for the $j$-th layer.

$$\mathbf{H}_j^{\mathrm{eff}} = K m_j^z \hat{\mathbf{z}} + A\nabla^2 \mathbf{m}_j + D\left[\left(\nabla \cdot \mathbf{m}_j\right)\hat{\mathbf{z}} - \nabla m_j^z\right] - J\mathbf{m}_{\underline{j}}$$

is the effective field acting locally on sub-layer $\mathbf{m}_j$, with $\underline{j}$ denoting the neighboring layer of $j$-th layer. The parameters are taken as following: the perpendicular easy-axis anisotropy $K = 3.88\times10^4$ A/m, the exchange coupling constant $A = 3.28\times10^{-11}$ A·m (*4, 9*), the coefficient of interfacial Dzyaloshinskii-Moriya Interaction (DMI) $D = 1.4\times10^{-3}$ A (*6*), and the antiferromagnetic exchange coupling due to RKKY interaction in the logic track is $J = 1.0\times10^6$ A/m. These values all fall into the

reasonable range of conventional SyAF structures (*10*). The effect of the dipolar fields can be neglected because of two reasons: i) the logic track is made of SyAF, whose dipolar fields are negligible, ii) the spin waves used are exchange spin wave with very short wavelength for which the long-range dipolar interaction can be ignored. Clocked current pulses (interval 10 ns, duration 0.8 ns) are applied in the memory track to shift the memory bit in the racetrack. The current-induced spin transfer torque in the memory track is taken as $\boldsymbol{\tau}_3 = (\mathbf{u} \cdot \nabla)\boldsymbol{m}_3 - \beta \boldsymbol{m}_3 \times (\mathbf{u} \cdot \nabla)\boldsymbol{m}_3$ (*11, 12*), where $\mathbf{u} = u_0 \hat{e}_y$ with $u_0 = \pm 500$ m/s represents the current flowing in certain direction $\hat{e}_y$ (in $\mp\mathbf{y}$ direction for the current in input/output track in Fig. 2). The Gilbert damping $\alpha_{1,2}$ in the logic track is taken as $4\times10^{-4}$, for which the spin wave can propagate up to 10 μm, sufficient for the purpose of logical operation considered in this paper. The damping constant is set to $\alpha_3 = 0.2$ (*13*) in the memory track to guarantee the stability of current-driven domain wall motion, and the non-adiabatic coefficient is $\beta = 0.2$. The exact value of $\beta$ is not crucial in this work.

<u>Parameters of the Spin Wave Logic Gates</u>

The width of the logic track is 200 nm, and the width of the memory track is $l =$ 240 nm. In this tri-layer retarder structure, the antiferromagnetic exchange coupling between the memory track and the logic track is $2J' = 1.35 \times 10^4$ A/m.

In the writing region, an asymmetric coupling between the logic track and the memory track is built in, *i.e.* the magnetization in the logic track can be easily imprinted into the memory track, while magnetization in the memory track has little effect on the magnetization in the logic track. Such effect can be realized by various approaches. One way is to make the total magnetization of the output memory track at crossing section much smaller than that of the logic track, which can be realized by either reducing the memory track thickness or using softer magnetic materials in the memory track.

The domain wall in the logic track has two stable positions: $P_1$ and $P_2$. $P_1$ is its natural position in the absence of driving forces (from injected spin wave), and $P_2$ is

the position when there is sufficient driving force. Such domain wall motion behavior is realized by building in an anisotropy gradient between $P_1$ and $P_2$ in the logic track. $P_1$ is the location with the minimum magnetic anisotropy. And the slope of the gradient defines the minimum force required for the domain wall being pushed to $P_2$. Such anisotropy gradient can be realized experimentally by various means, e.g. by ion irradiation (*15*) or geometric thickness/width modulation. (*16*) (*17*) In our simulation, the anisotropy gradient is taken as $2\times10^9$ A/m$^2$. When the driving force due to the reflected spin wave overcomes the anisotropy gradient, the domain wall moves to position $P_2$.

The force exerted by the spin waves depends on the frequency, amplitude and the polarization of the spin wave, the strength of DMI, and so on (*7*). By taking account of the efficiency of magnetic gating effect and the polarization-selective domain wall motion, the frequency of injected spin waves is chosen as $f = 11$ GHz, and the rotation angle of $+29/-16°$ is obtained for magnetic bit '0'/'1' in the memory track.

The spin wave amplitude is chosen corresponds to a magnetization cone angle of 5.7 degrees. This spin wave amplitude can be reduced if we add an assisting electric current in the logic track that moves the domain wall from $P_1$ to $P_2$.

## 2. Logic gates based on double-threshold nonlinearity

A Boolean logic maps an $n$-bit input to an 1-bit output. When treating the input and output bits in equal foot, there are $n + 1$ possible bits, thus in total $2^{n+1}$ different types of gates. Two of them are trivial gates which unanimously map all inputs to 0 (or 1), and the rest $2^{n+1} - 2$ gates are non-trivial logic gates. For example, there are 2 non-trivial unary gates ($n = 1$): the CLONE and NOT gate, and there are 6 non-trivial binary gates ($n = 2$): the AND, OR, XOR, NAND, NOR, XNOR gate.

In order to realize logic gates, physical systems with non-linearity are required. A typical nonlinear physical behavior is the threshold behavior, *i.e.* some physical

property undergoes an abrupt change when the input is above certain threshold (see Figure S3).

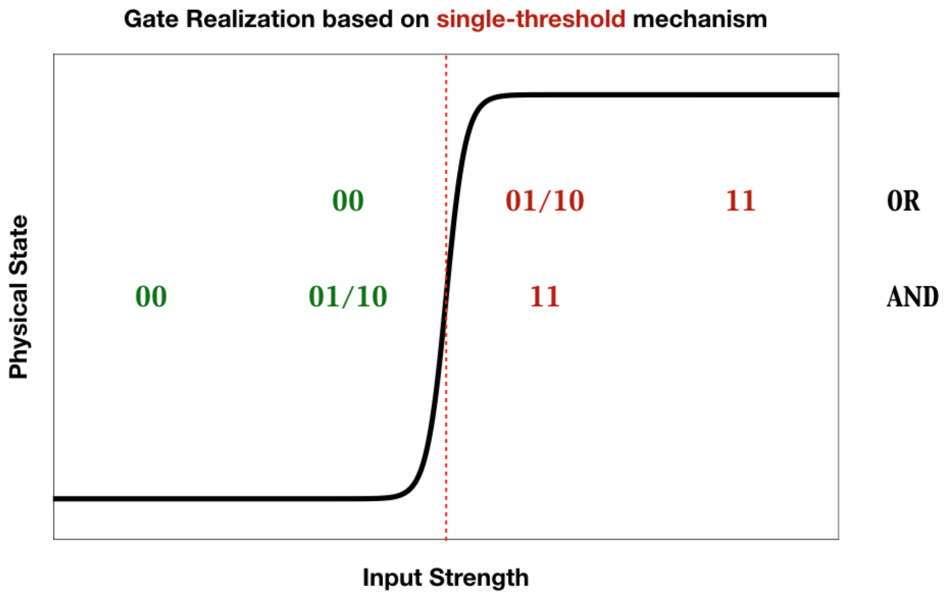


**Fig. S3.** *Logic Gate realization based on a single threshold mechanism.*

Typically, the strength of the input is a monotonic function of number of 1s in the input. Therefore, the input strength increases in sequence of 00, 01/10, 11. When the threshold is set to be between 00 and 01/10, it distinguishes 00 from 01/10 and 11 and realizes an OR gate. When the threshold is between 01/01 and 11, it realizes an AND gate. However, the single threshold behavior cannot realize the XOR gate, which distinguishes input 01/10 from 00 and 11.

The non-linearity used in this paper shows a special double-threshold behavior, *i.e.* the physical state undergoes an upward abrupt change when the input strength saturates, and undergoes another downward abrupt change when the input strength oversaturates. The physical systems with such double-threshold behavior can not only realize the OR and AND gate, but also the XOR gate, as shown in Fig. S4.

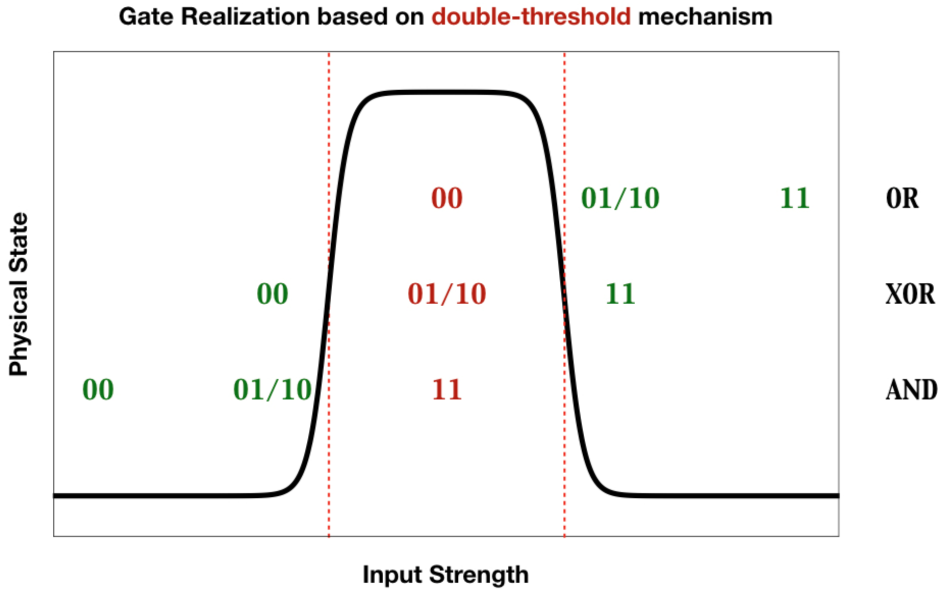


**Fig. S4.** *Logic Gate realization based on a double threshold mechanism.*

In this paper, the input is the polarization angle of the spin wave. The domain wall moves forward only if the polarization angle $\theta$ is close to 90 degrees (or $|\sin\theta| \approx 1$), while the domain wall does not move when the polarization angle is much smaller or larger than 90 degrees (e.g. $|\sin\theta| < 0.5$), thus realizing a double-threshold behavior as required.

Typically, the input strength is not easily tunable, thus the threshold value needs to be adjusted to realize different gates, no matter it is for the single-threshold or double-threshold systems. Therefore, different gates would need different hard structures. However, for the spin wave logic in this paper, the threshold values keep unchanged, but the input strength (polarization angle here) can be easily modulated via tuning the initial polarization angle. Because of the double-threshold behavior and the polarization tunability, the spin wave logic gate is a universal logic gate, *i.e.* one hardware structure realizes all logic functionalities.

## 3. Fulfillment of five essential characteristics for scalable computing

For a computing architecture to be fully functional and scalable, it has to meet the above five requirements: non-linearity, Boolean functions, feedback elimination,

gain and concatenability. As for the present spin wave logic, the "nonlinearity" naturally comes from the double-threshold behavior of polarized-spin-wave driven domain wall motion in the logic track. Apparently, the spin wave logic here can realize all "Boolean functions", and in fact, using only one hard structure. "Feedback elimination" is ensured because the domain wall in logic track is constrained between P1 and P2 by gradient anisotropy, thus its influence is not able to penetrate back into the input memory track. There is no "gain" issue neither, because the power is supplied through spin wave injection in each logic track (via microwave through micro-antenna or spin current for instance), thus no gain from the input track is needed. And since both input and output of the logic are racetrack memories, the spin wave logic automatically possesses the "concatenability" by using the output track of one logic gate as the input track of the following logic gates.

## 4. Operation Steps of 4-bit Adder

In this supplementary material, we demonstrate the arithmetic operation ADD WITH CARRY of a 4-bit ALU. In the example, the 4-bit input is 1011 and 0111 with an additional carry. The spin wave injection in logic track and electric current in the memory track are both pre-programmed for the ADD operation. The calculation is iterated for four times and finally outputs the right result with the right carry. The calculation steps are shown in Fig.S1 and Fig.S2. Movie S4 demonstrates the time-dependent process.

| | | | | | | |
|---|---|---|---|---|---|---|
| Addition with Carry-in and Carry-out | 1011 + 111 + 1 = 10011 | | | | | |
| | | 1 | 0 | 1 | 1 | Input A |
| | | 0 | 1 | 1 | 1 | Input B |
| | + | | | | 1 | Carry-in |
| Carry-out | 1 | 0 | 0 | 1 | 1 | Output |

| Iteration | | | | | | | | | | | | | | |
|---|---|---|---|---|---|---|---|---|---|---|---|---|---|---|
| | Input A, Carry-in | | | | | | 1 | 0 | 1 | 1 | 0 | 1 | 0 | 0 |
| | Input B | | | | | | 0 | 1 | 1 | 1 | | | | |
| 1 | Carry | A AND B | | | | 0 | 0 | 1 | 1 | 0 | 1 | 0 | 0 | |
| | Sum | A XOR B | | | | | 1 | 1 | 0 | 0 | | | | |
| 2 | Carry | A AND B | | | 0 | 0 | 1 | 0 | 0 | 1 | 0 | 0 | | |
| | Sum | A XOR B | | | | | 1 | 0 | 1 | 0 | | | | |
| 3 | Carry | A AND B | | 0 | 0 | 1 | 0 | 0 | 0 | 0 | 0 | | | |
| | Sum | A XOR B | | | | | 0 | 0 | 1 | 1 | | | | |
| 4 | Carry | A AND B | 0 | 0 | 1 | 0 | 0 | 0 | 0 | 0 | | | | |
| | Sum | A XOR B | | | | | 0 | 0 | 1 | 1 | | | | |
| | Carry | A AND B | 0 | 0 | 1 | 0 | 0 | 0 | 0 | 0 | | | | |
| | Sum | A XOR B | | | | | 0 | 0 | 1 | 1 | | | | |
| | Carry-out | | 0 | 0 | 1 | 0 | 0 | 0 | 0 | 0 | | | | |
| | Sum | | 0 | 0 | 1 | 1 | | | | | | | | |

**Fig. S5.** *Principle of the operation ADD WITH CARRY. The input information are 1011 and 0111 (red region), the carry is 1 (yellow region). In each iteration, there will be a bit of carry involved into the adding operation. After four iterations, the calculated result is converged. The final result is the 0011 (red) with the carry-out 1 (yellow). For our device, it is defined that 1000/0100/0010/0001 represents carry 1 while 0000 represents carry 0.*

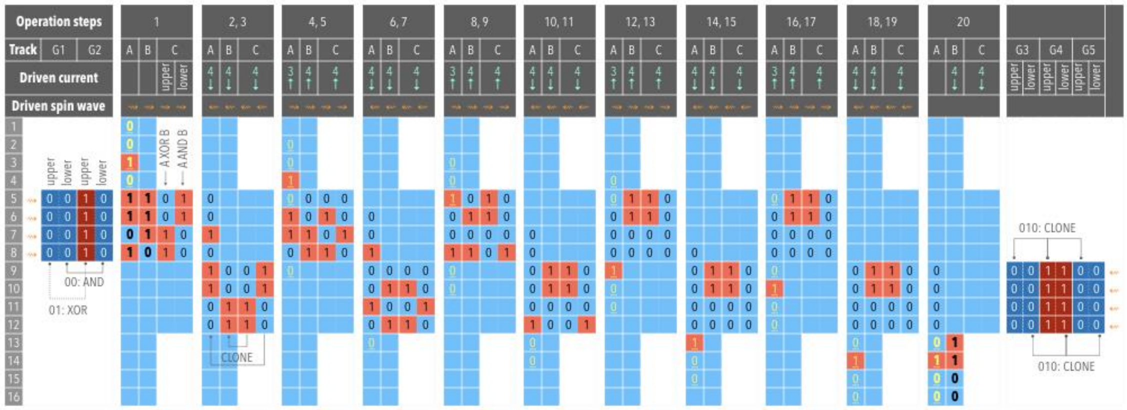


| | | |
|---|---|---|
| 4-bit Full Adder | Performing addition for inputs A = 1011 and B = 0111 with carry-in 1, the output is 0011 with carry-out 1, i.e. 1011 + 0111 = 10011. The inputs/outputs and carry-in/out are in **bold** in step 1/20. | |
| Carrys | The carry-in and carry-out bits are underlined. At most one out of the four carry bits can be 1, and the carry 1000, 0100, 0010, 0001 all represent carry-in 1. | |
| Step 1 | Driving spin wave in the forward logic wires (pos. 5- 8) | Performing logic operation (XOR and AND) on input track A, B, writing results into track C: $C_{upper}$ = A XOR B, $C_{lower}$ = A AND B |
| Step 2 | Driving current in track A, B, C from top | Shifting the racetrack memories in A, B, C down by 4 positions to pos. 9-12 |
| Step 3 | Driving spin wave in the backward logic wires (pos. 9- 12) | Copying the bits in track C back into track A and B: A = $C_{lower}$, B = $C_{upper}$ |
| Step 4 | Driving current in track A, B, C from bottom | Shifting memory track B up by 4 positions and track A by 3 positions (shifting by 1 position relative to B, thus annexing one carry-in bit to pos. 5) |
| Step 5 - 19 | Repeating Step 1 - 4 four more times | Annexing one carry-in bit each time |
| Step 20 | Driving current in track B from top | Shifting memory track B down by 4 positions, the final result is stored in track B and the carry-out in track A (pos. 13- 16) |

**Fig. S6.** *Schematics of the operation ADD WITH CARRY.*

## 5. Descriptions for Movies S1 to S3

**Movie S1**: Micromagnetic simulation of the 1-bit NOT gate. The injected spin waves are 106° polarized. All the parameters are consistent with those listed in Numerical Method. The simulation duration is 40 ns so that there are 4 operations demonstrated.

**Movie S2**: Micromagnetic simulation of the 2-bit OR gate. The injected spin waves are 32.5° polarized. All the parameters are consistent with those listed in Numerical Method. The simulation duration is 50 ns so that 5 operations are demonstrated. The demonstration covers the full cycle of 2-bit truth table and is proven to work as an OR gate as shown in Fig. 3 in the main text.

**Movie S3**: Micromagnetic simulation of the 4-bit universal gate. The injected spin waves are 90° polarized (linear-y polarization). The Gilbert damping is reduced to $3.6\times10^{-4}$ to compensate the additional propagation length induced by the instruction tracks. The simulation duration is 120 ns so that 12 operation are demonstrated. The 12 operations cover the full cycle of 2-bit truth table ($2^2$=4 operations) three times. According to different instructions 11/00/01, the universal gate works as OR/NAND/XNOR respectively which is consistent with Fig.4 in the main text.

## References

1. H. Szambolics *et al.*, Innovative Weak Formulation for the Landau–Lifshitz–Gilbert Equations. *IEEE Transactions on Magnetics* **44**, 3153-3156 (2008).
2. F. Alouges, E. Kritsikis, J.-C. Toussaint, A convergent finite element approximation for Landau–Lifschitz–Gilbert equation. *Physica B: Condensed Matter* **407**, 1345-1349 (2012).
3. COMSOL Multiphysics, http://www.comsol.com.
4. J. Lan, W. Yu, R. Wu, J. Xiao, Spin-Wave Diode. *Physical Review X* **5**, 041049 (2015).
5. W. Yu, J. Lan, R. Wu, J. Xiao, Magnetic Snell's law and spin-wave fiber with Dzyaloshinskii-Moriya interaction. *Physical Review B* **94**, 140410 (2016).
6. J. Lan, W. Yu, J. Xiao, Antiferromagnetic domain wall as spin wave polarizer and retarder. *Nature Communications* **8**, 178 (2017).

7. W. Yu, J. Lan, J. Xiao, Polarization-selective spin wave driven domain-wall motion in antiferromagnets. *Physical Review B* **98**, 144422 (2018).
8. R. Cheng, J. Xiao, Q. Niu, A. Brataas, Spin Pumping and Spin-Transfer Torques in Antiferromagnets. *Physical Review Letters* **113**, 057601 (2014).
9. P. Yan, X. S. Wang, X. R. Wang, All-Magnonic Spin-Transfer Torque and Domain Wall Propagation. *Physical Review Letters* **107**, 177207 (2011).
10. R. A. Duine, K.-J. Lee, S. S. P. Parkin, M. D. Stiles, Synthetic antiferromagnetic spintronics. *Nature Physics* **14**, 217-219 (2018).
11. Z. Li, S. Zhang, Domain-Wall Dynamics and Spin-Wave Excitations with Spin-Transfer Torques. *Physical Review Letters* **92**, 207203 (2004).
12. S.-M. Seo, K.-J. Lee, H. Yang, T. Ono, Current-Induced Control of Spin-Wave Attenuation. *Physical Review Letters* **102**, 147202 (2009).
13. Y. Zhou, M. Ezawa, A reversible conversion between a skyrmion and a domain-wall pair in a junction geometry. *Nature Communications* **5**, 4652 (2014).
14. R. Cheng, M. W. Daniels, J.-G. Zhu, D. Xiao, Antiferromagnetic Spin Wave Field-Effect Transistor. *Scientific Reports* **6**, 24223 (2016).
15. J. H. Franken, H. J. M. Swagten, B. Koopmans, Shift registers based on magnetic domain wall ratchets with perpendicular anisotropy. *Nature Nanotechnology* **7**, 499 (2012).
16. S. Li *et al.*, Magnetic skyrmion-based artificial neuron device. *Nanotechnology* **28**, 31LT01 (2017).
17. X. Chen *et al.*, A compact skyrmionic leaky-integrate-fire spiking neuron device. *Nanoscale* **10**, 6139-6146 (2018).
